# Supplementary material for: Hunting for the progenitor of SN 1006: High resolution spectroscopic search with the FLAMES instrument
Source: arXiv:1207.4481 source file (2012-07-18)
Supplement: Supplementary file 1 [file chapter_sn1006_appendix.tex]

\chapter{SN 1006 Data}
\input{chapter_sn1006/tables/phot_table}
\newpage
\input{chapter_sn1006/tables/phot_2mass_table}
\newpage
\input{chapter_sn1006/tables/kinem_table}
\newpage
\input{chapter_sn1006/plots/gold_spectra/images}
